# Supplementary material for: Identifying Disinformation Websites Using Infrastructure Features
Source: arXiv:2003.07684 source file (2020-09-28)
Supplement: Supplementary file 2 [file foci-appendix.tex]

\section{Appendix: Classifier Features}
\label{apx:features}
\input{figures/features_table}
